# Supplementary material for: Diagnostic Prediction Using Discomfort Drawings with IBTM
Source: arXiv:1607.08206 source file (2016-09-13)
Supplement: Supplementary file 1 [file appendix.tex]

\section{Appendix}

{
\scriptsize
\begin{table}[h]
\centering
\scriptsize
\begin{tabular}{ | c  | c || c | c|}
\hline
Swedish	& Englsh&
Swedish	 & Englsh  \\
\hline	
 Achillesbesv\"ar & Achilles discomfort  &
 Achillestendalgi & Achilles tendinitis \\
 Acromio Cavikular skada&Acromioclavicular damage &
 Achillodyni &Achillodynia \\
Acromio Clavikular  & Acromioclavicular &
Adduktortendalgi & Adductor tendonitis \\
Adduktorskada& Adductor injury &
 Armbesv\"ar & Arm discomfort \\
 Armb\aa gsbesv\"ar & Elbow discomfort &
Armveckbesv\"ar& Bend of the arm discomfort \\
Axelskada& shoulder  injury&
Axel impingement & Shoulder impingement\\
Bakhuvudvärk & Back headache &
 Bakre l\aa rbesvär & Back thigh discomfort \\
Bechterew& Bechterew's Disease&
Bicepstendalgi & Biceps Tendalgi\\
Bicepsskada& Biceps Injury&
Br\"ostbesv\"ar & Chest discomfort \\
Bröstryggsbesv\"ar &Thoracic spine discomfort &
Bukbesv\"ar & Abdominal discomfort \\
Benbesv\"ar & Leg discomfort &
 Central br\"ostsm\"arta & Central chest pain \\
 Centrala br\"ostbesv\"ar & Central chest discomfort &
Carpaltunnelsyndrom & Carpal tunnel syndrome\\
Centrala Ljumskbesv\"ar &Central groin discomfort &
Coccyxdyni & coccydynia\\
Coccyxskada & coccyx damage&
Coxartros & coxarthrosis\\
Coxysskada &  coccyx osteoarthritis&
DLS & discolegament injury \\
DLS spinalstenos & discolegament injury spinal stenosis&
Fasettskada& Facet damage\\
%Fasettledsbesv\"ar & Facet joints discomfort &
%Fasettledskada &Facet joint damage \\
Fibromyalgi & Fibromyalgia&
 Fingerbesv\"ar & Finger discomfort \\
 Fotbesv\"ar & Fot discomfort &
 Fotledbesv\"ar & Ankle  discomfort \\
 Fotvalvsbesv\"ar & Arch discomfort &
Fotledsdistortion &Ankle sprain \\
Fotledsskada &Ankle Injury  &
Fraktur Metatarsale 5 &Fracture Metatarsale 5 \\
 Fr\"amre kn\"abesv\"ar & Anterior knee discomfort &
 Fr\"amre l\aa rbesv\"ar &   Front thigh discomfort \\
 Hamstringsb & Hamstrings discomfort &
 Handbesv\"ar & Hand discomfort \\
 Handledsbesv\"ar& Hand joint discomfort &
Handlesganlion & Hand joint ganglion \\
Huvudv\"ark & Headache &
 H\"albesv\"ar & Calcaneal pain \\
 H\"oftbesv\"ar & Hip discomfort &
 H\"oftkamsbesv\"ar &  Crest of the ilium discomfort \\
IBS & Irritable Bowel Syndrome&
Interskapulära besv\"ar & Interscapular  discomfort \\
 Ischias & Sciatica &
 Kn\"abesv\"ar & Knee discomfort \\
 K\"akbesv\"ar & jaw discomfort &
Kn\"a sk\aa lsskada & patellar Injury \\
Kondromalacia patella & Chondromalacia Patella &
Kraniocervikal ledskada & craniocervical joint injury\\
Fasettledskada & Gacet joint injury&
Fasettledsbesv\"ar & Gacet joint discomfort \\
Gastrocnemiusbesvär &Gastrocnemius discomfort &
Kraniocervikal ledskada &craniocervical joint injury \\
Labrumskada & Glenoid damage&
 Laterala Fotbesvär &   Lateral fot discomfort \\
 Laterala armb\aa gsbesvär & Lateral elbow discomfort &
 Laterala armsbesv\"ar &  Lateral arm discomfort \\
Laterala bukbesv\"ar & Lateral abdominal discomfort &
 Laterala knäbesv\"ar & Lateral knee  discomfort \\
 Laterala ljumskbesv\"ar & Lateral groin discomfort &
 Laterala vadbesv\"ar & Lateral lower leg  discomfort \\
%Labrumskada & Glenoid damage &
% Lillfingerbesv\"ar & Littlefinger  discomfort \\
 Lillt\aa besv\"ar &  Little toe discomfort &
 Ljumskbesv\"ar & Groin discomfort\\
Ljumskbr\aa ck & inguinal &
 Lumbago & lumbago \\
 L\aa rbesv\"ar & Thigh  discomfort &
Lateral Fotledsbesv\"ar & Lateral ankle discomfort  \\
Lateral gonartros &Lateral gonarthrosis &
Ljumskbr\aa ck &Inguinal \\
Medial Menisk & Medial Meniscus &
Medial Meniskskada &Medial meniscus injury \\
Medial gonartros &Medial gonarthrosis &
Medial kn\"aartros &Medial knee osteoarthritis \\
Medial menisk &Medial meniscus &
Medial menisk ruptur & Medial meniscal rupture\\
 Mediala armb\aa gsbesvär & Medial elbow discomfort &
Mediala kn\"a ledsbesvär & Medial knee joint discomfort \\
 Mediala ljumskbesvär & Medial  groin discomfort &
Meniskskada & Meniscal Injury \\
Munbesv\"ar &Mouth discomfort &
Muskelspänning & Muscle tension\\
Nackbesv\"ar & Neck discomfort &
Nedre bukbesv\"ar & lower abdominal discomfort \\
Nerv Stam & Nerve Strain &
Nervstamsp\aa verkan & Nerve Strain Effect\\ 
 Nyckelbensbesv\"ar &  Collarbone  discomfort &
OB & Cannot be decided\\
Ospecifik Armbesvar & Nonspecific Arm discomfort &
 PFS & Patellofemoral pain syndrome \\
 Pannhuvudvärk & Forehead Headache &
Partiell bicepsseneruptur &Partial biceps tendon rupture \\
Prepatell\"ar Artros & Osteoarthritis prepatellar &
Radikulopati & Radiculopathy\\
%Ryggradsbesvär & Spine discomfort
%Ryggsbesvär & Backache
% Skinkbesvär & upper side leg discomfort
% Skulderbesvär & inner shoulder  discomfort
Schlatter &Schlatter disease &
Spinalstenos & Spinal stenosis\\
Spondylolistes  & Spondylolisthesis &
Suprastinatuskada &Supraspinatus injury \\
%Stort\aa skada & Big toe Injury &&\\
Tibiaperialgi & shin discomfort &
 Tinnitus & Tinnitus  \\
% Tumbesvär & Thumb discomfort
% Tåledbesvär & Ankel discomfort
% Tårbesvär & Toe  discomfort
Titze sydrom & Titze syndrome &
Torakal Dysfunktion & Thoracic dysfunction \\
% Under armsbesvär & Lower arm  discomfort
% Underbensbesvär & Lower leg  discomfort
% Vadbesvär & lower back leg  discomfort
% Ögonbesvär & Eye  discomfort 
% Öronbesvär& ear  discomfort 
% Övre armbågsbesvär & Upper elbow discomfort 
% Övre armsbesvär & Upper arm Elbow discomfort
%Övre bukbesvär & Upper abdominal discomfort
\hline
\end{tabular}
\caption{List of Swedish - English dictionary of medical terms in paper}
\label{tab:Exchange}
\end{table}
}
